# Supplementary material for: YaART: Yet Another ART Rendering Technology
Source: arXiv:2404.05666 source file (2024-04-08)
Supplement: Supplementary file 1 [file 11_appendix.tex]

\section{Limitations}
% \label{sec:limitations}
Contrary to main stream approach to training text to image diffusion models as LDMs, we have chosen the cascaded diffusion variant. Even though the it requires  more computational resources at runtime there are benefits from the more interactive nature of cascaded generation: we can provide the 256x256 image for further filtering and refining by the user; the superresolution stage is only applied to a fraction of the generated images, which were selected by the user. 
Altogether we have come to the conclusion that, despite all the recent progress in this area, modern diffusion models still necessitate substantial human supervision. This typically involves iterative prompt modification, sampling parameter tuning (or even adjusting the random seed), and a post-filtering process for the generated images. 

We have also applied automatic filters to eliminate images containing text from our dataset. We made this decision because we believe the quality of text generation is insufficient for practical use cases. Interestingly our model still learned to generate reasonable characters and words from the limited amount of images contraining text, that remained in our training dataset.

\section{Additional images}
\label{sec:add-imgs}

Supplementary materials do not get included in the initial submission (there is yet another deadline for that) but we still can place them here now if we are sure that these things should not be a part of the main text.

\begin{figure}[tp]
  \centering
  \includegraphics[width=0.48\textwidth]{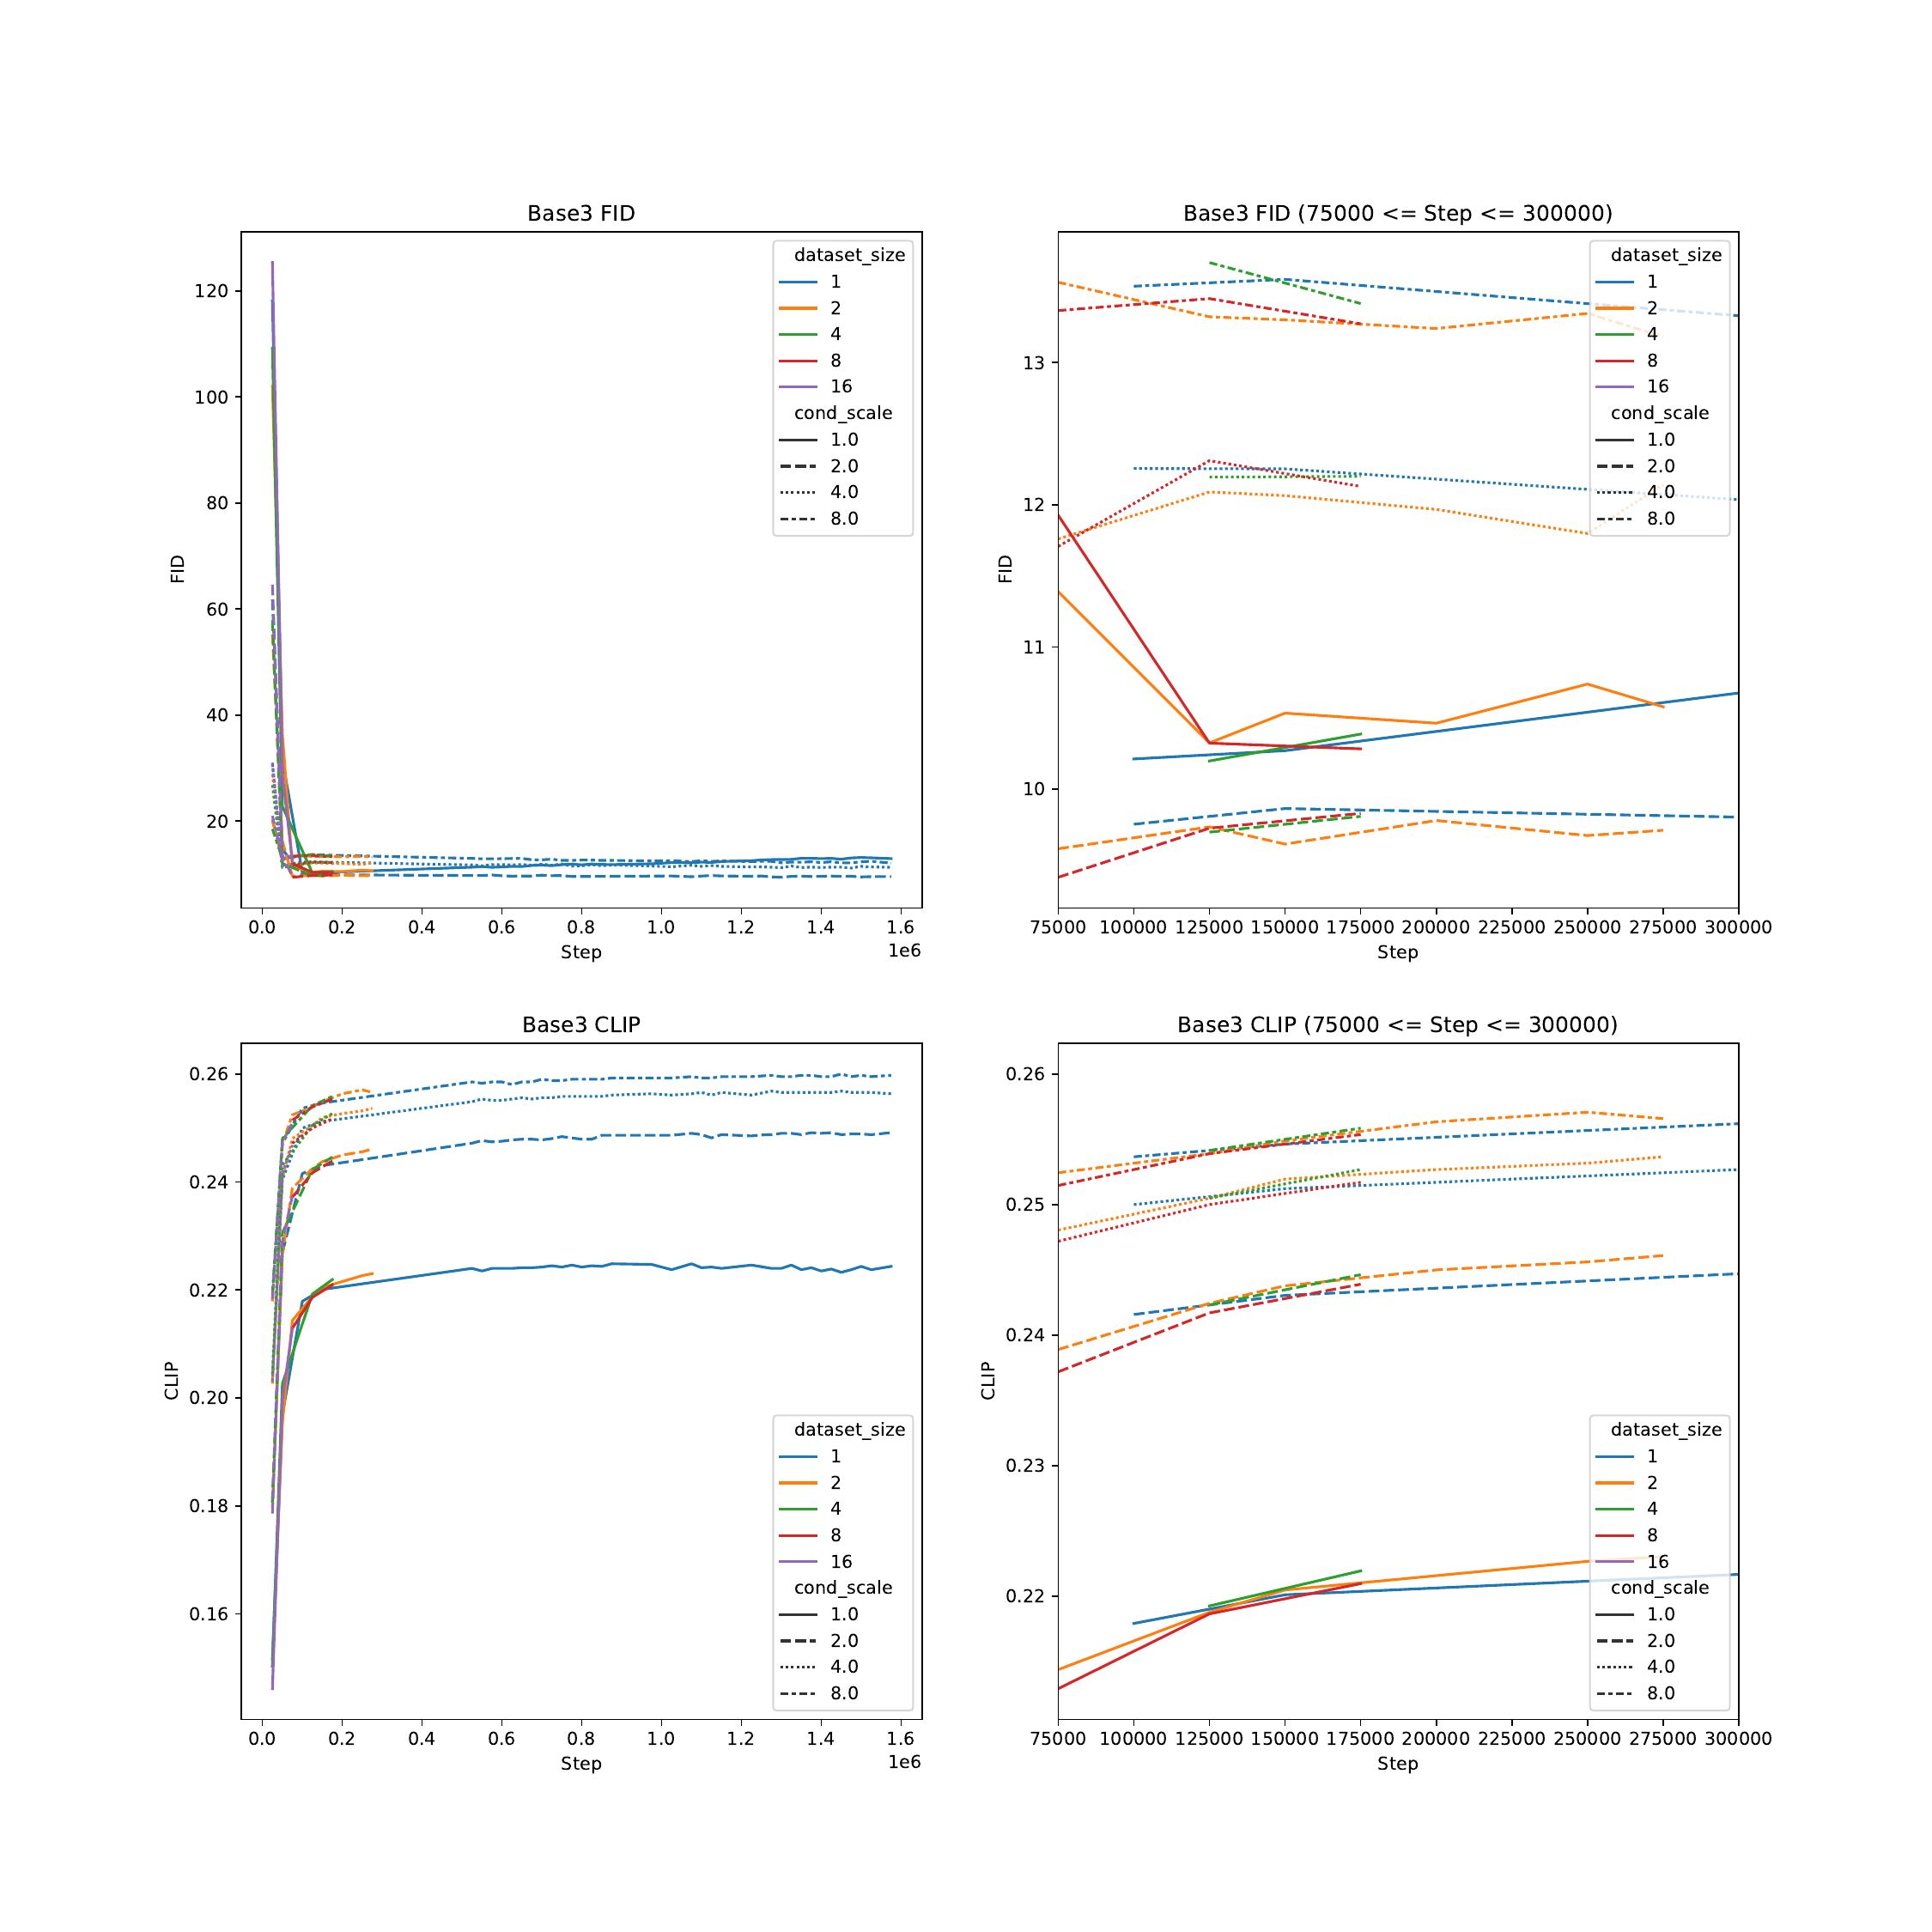} 
  \caption{FID/CLIP curves}
\end{figure}

\begin{figure}[tp]
  \centering
  \includegraphics[width=0.48\textwidth]{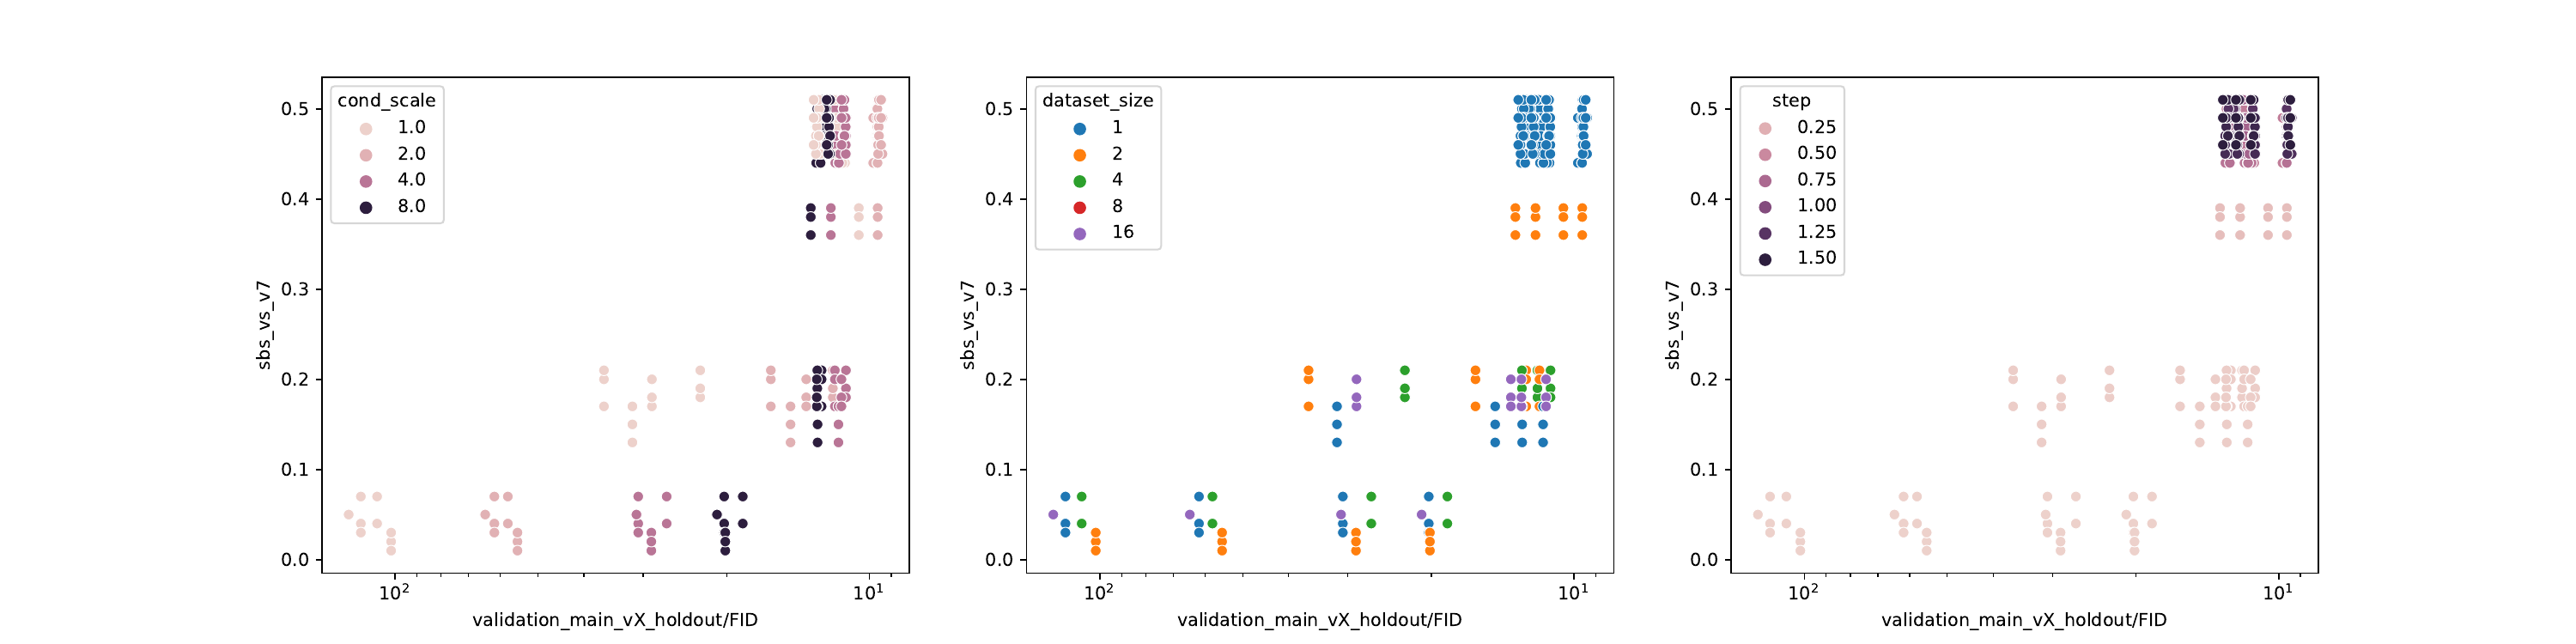} 
  \caption{SbS and FID}
\end{figure}

\section{More figures and tables}
\label{sec:figs-and-tabs}
