# Supplementary material for: YaART: Yet Another ART Rendering Technology
Source: arXiv:2404.05666 source file (2024-04-08)
Supplement: Supplementary file 2 [file 04_fid_sbs.tex]

\section{FID and Human Evaluations}
\label{sup:fid_sbs}

Our research does not rely on the Fréchet Inception Distance (FID) metric for evaluating the quality of generated images due to its low correlation with human evaluation when a generative model already produces high-quality results. This limitation of the FID metric has been acknowledged in previous works (SD XL, ???) and our study aligns with these findings (see Figure {}).

Caption for figure: The evolution of FID scores and human assessment scores during the training of a 1.4B sized model on full dataset. Despite a consistent change in FID scores throughout the training process, there is no corresponding change in human evaluation scores, demonstrating the disconnect between the two metrics in assessing the quality of generated images.
